# Supplementary material for: Precision Studies of QCD in the Low Energy Domain of the EIC
Source: arXiv:2211.15746 source file (2023-02-10)
Supplement: Supplementary file 1 [file Additional.tex]

\section{Additional text- not to be fully included }

{\color{blue} \underline{V.B.}:{\bf {\color{blue} Some alternate thoughts on the "mass" topic and on emergent mass. This is not meant as a
contribution to the text, but as a point of discussion. Mass of matter is not a fixed number but changes with temperature. These processes are being studied at RHIC by energy scans (changing temperature in the plasma). } It would be nice to have some discussion of this, maybe in an introduction. It may allow connecting studies of heavy ion collisions and of the EIC science.} }  \\

{\color {blue} V.B.: As scientist we not only want to understand the universe as it is, but also how it evolved from 
the Big Bang 
through various phase transitions to the present time. 
Just microseconds after it came into existence, the universe entered in a crossover period from the quark-gluon plasma 
phase to the hadron phase that was characterized by a cool down to the few-hundred MeV temperature range, 
accompanied by the emergence of hadron resonances, the occurrence of chiral symmetry breaking and the 
emergence of confinement and stable baryons. This is being studied in hot-LQCD simulations.The transition 
temperature appears to be near 155 MeV. These processes are currently 
being studied experimentally at RHIC in high-energy heavy ion collisions with the ongoing energy scan. The large gap  
between hot-LQCD and hadron resonance models that include known strange- charmed-states, show that many hadrons 
carrying strange and charm flavors are still 
to be found to solve part of the missing baryon pressure gap in Fig.\Ref{universe}. 
The EIC could play a very important role in their discovery, especially in the charmed quark sector.   \\
\begin{figure}[h] 
\hspace{-0.2cm}\includegraphics[width=0.34\columnwidth]{figures/universe_chronology.jpg}
\hspace{1.0cm}\includegraphics[width=0.40\columnwidth]{figures/strange-charm-pressure.png}
\caption{Chronology of the evolution of the universe (left). The crossover from the quark-gluon plasma 
phase to the hadron phase (right) takes place at about 1$\mu$sec, with the critical temperature near 155 MeV. 
Markers show Lattice calculations for strange and charm baryon/meson versus temperature from weekly 
interacting quarks at high temperatures to near bound quarks below 150 MeV. Lines indicate hadron gas 
model calculations with hadron states as tabulated in RPP20xx and hadrons from full quark model. 
Lines do not fit the hot-LQCD results, indicating significant amount of missing baryons pressure of 
strange and charm flavor. Similar but lower missing baryon pressure is observed for light-quark baryons.} 
\label{universe}
\end{figure}

\noindent How can we study the emergence of hadron rest masses at the EIC? 
It has been known for some time that the fundamental Higgs mechanism~\cite{Higgs} leads to masses of 
elementary quarks. 
However, in the light-quark sectors of u-quarks and d-quarks such as the nucleon and its excitation spectrum 
in the baryon sector, and light unflavored mesons such as the $\pi$, $\rho$ and their excitation  
in the meson sector, elementary quark masses $\rm m_q$ contribute only a few MeV to the hadrons rest mass $\rm M_h$, 
leaving much of $\rm M_h$ to be generated by the gluons and their dynamical interactions with the 
quarks and with other gluons to give rise to the quark's "constituent" mass $m_Q$ of several hundred MeV/c$^2$.  delete. xji}

{\color{red} XJI: this is a wrong picture for mass. There is
a mass scale $\Lambda_{QCD}$, quark kinetic energy will
generate large contribution to the mass, gluon has the standard energy contribution as $E^2 + B^2$}. {\color{green} VB: How do gluons factor into that picture? gluon has the standard energy contribution as $E^2 + B^2$ }\\

{\color{blue} The model of a "constituent" quark mass $\rm m^Q$ has been shown in light-cone relativistic quark model~\cite{Aznauryan} with 
running quark mass, and in continuum QCD related studies~\cite{Segovia}, not to be constant, but to depend on
the distance scale at which the proton's structure is probed, e.g. in elastic scattering and in resonance 
excitation processes at high photon virtuality. Virtual photons in the range $Q^2 > 50$GeV$^2$ will be 
required to begin seeing the transition effect of elementary quark interaction as is shown in Fig.~\ref{fig-x}.
With increasing photon virtuality the gluon cloud is increasingy penetrated and probes closer to the 
elementary mass. If expressed in reverse order, by probing the quarks at smaller $Q^2$, the quarks begin to 
get dressed increasingly with gluons leading to increasingly higher effective masses. In analogy to the evolution 
of the universe, or high-energy heavy ion collisions, it corresponds to the hadron mass emerging at lower temperature, 
or lower energy transfer. \\

The dynamics of the emerging hadron mass could be studied best in measurement in the valence 
quark regime and at elastic processes $ep \to ep$ and resonance transitions in $ep \to e\pi^+ n, eK^+\Lambda, ep \pi^+\pi^-$ and other reactions at high $Q^2$, focusing on the $x_B > 0.05 $ range. This requires highest luminosity at low CM energies. 
The kinematics at lowest CM energy is shown in shown in Fig.~\ref{EIC-kine1}. } \\
